# Supplementary material for: Extended Object Tracking Using Sets Of Trajectories with a PHD Filter
Source: arXiv:2109.01019 source file (2021-09-02)
Supplement: Supplementary file 1 [file Appendix_1.tex]

% CREATED BY DAVID FRISK, 2018
\chapter{Appendix 1}
\label{ch:Appendix_1}

\section{Pseudocode for GGIWPHD filter pruning, merging and capping}
\begin{table}[ht]
\caption{Pseudocode for GGIWPHD filter pruning, merging and capping}
\rule{\textwidth}{0.5pt}
\begin{algorithmic}[1] \label{GGIWreduction}
    \STATE \textbf{input:} GGIW components $\left\{w_{k|k}^{(j)}, \xi_{k|k}^{(j)}\right\}_{j=1}^{J_{k|k}}$, a pruning threshold $T$, a merging threshold $U$ and a maximum number of allowed components $M$.
    \STATE \textbf{init:} Set $\ell \gets 0$ and $I \gets \left\{ i=1,...,J_{k|k} \big| w^{(i)}_{k|k} > T ~\land~ \frac{\alpha^{(i)}_{k|k}}{\beta^{(i)}_{k|k}} > 1 \right\}$
    \REPEAT 
        \STATE{$\ell \gets \ell + 1$}
        \STATE{$j \gets \underset{i\in I}{\arg\max} ~ w^{(i)}_{k|k}$}
        % \STATE{ $\hat{P}^{(j)}_{k|k} \gets (Pj^{(j)}_{k|k})/(\nu^{(j)}_{k|k}+n-n*d-2)$}
        \STATE{$L \leftarrow\left\{i \in I \Big|\left(m_{k|k}^{(i)}-m_{k|k}^{(j)}\right)^{\mathsf{T}}\left(P_{k|k}^{(j)}\right)^{-1}\left(m_{k|k}^{(i)}-m_{k|k}^{(j)}\right) \leq U\right\}$}
        \STATE{$\tilde{w}_{k|k}^{(\ell)} \leftarrow \sum_{i \in L} w_{k|k}^{(i)}$}
        \STATE{$\tilde{\alpha}_{k|k}^{(\ell)} \leftarrow \frac{1}{\tilde{w}_{k|k}^{(\ell)}} \sum_{i \in L} w_{k|k}^{(i)} \alpha_{k|k}^{(i)}$}
        \STATE{$\tilde{\beta}_{k|k}^{(\ell)} \leftarrow \frac{1}{\tilde{w}_{k|k}^{(\ell)}} \sum_{i \in L} w_{k|k}^{(i)} \beta_{k|k}^{(i)}$}
        \STATE{$\tilde{m}_{k|k}^{(\ell)} \leftarrow \frac{1}{\tilde{w}_{k|k}^{(\ell)}} \sum_{i \in L} w_{k|k}^{(i)} m_{k|k}^{(i)}$}
        \STATE{$\tilde{P}_{k|k}^{(\ell)} \leftarrow \frac{1}{\tilde{w}_{k|k}^{(\ell)}} \sum_{i \in L} w_{k|k}^{(i)} P_{k|k}^{(i)}$}
        \STATE{$\tilde{\nu}_{k|k}^{(\ell)} \leftarrow \frac{1}{\tilde{w}_{k|k}^{(\ell)}} \sum_{i \in L} w_{k|k}^{(i)} \nu_{k|k}^{(i)}$}
        \STATE{$\tilde{V}_{k|k}^{(\ell)} \leftarrow \frac{1}{\tilde{w}_{k|k}^{(\ell)}} \sum_{i \in L} w_{k|k}^{(i)} V_{k|k}^{(i)}$}
        \STATE{$I \gets I\setminus L$}
    \UNTIL{$I = \emptyset$}
    \STATE If $\ell > M$ then replace $\left\{\tilde{w}_{k|k}^{(j)}, \tilde{\alpha}_{k|k}^{(j)}, \tilde{\beta}_{k|k}^{(j)}, \tilde{m}_{k|k}^{(j)}, \tilde{P}_{k|k}^{(j)}, \tilde{\nu}_{k|k}^{(j)}, \tilde{V}_{k|k}^{(j)}\right\}_{j=1}^{\ell}$ by those of the $M$ components with largest weights.
    \STATE \textbf{output:} $\left\{\tilde{w}_{k|k}^{(j)}, \tilde{\xi}_{k|k}^{(j)}\right\}_{j=1}^{\ell},\tilde{\xi}_{k|k}^{(j)}=\left(\tilde{\alpha}_{k|k}^{(j)}, \tilde{\beta}_{k|k}^{(j)}, \tilde{m}_{k|k}^{(j)}, \tilde{P}_{k|k}^{(j)}, \tilde{\nu}_{k|k}^{(j)}, \tilde{V}_{k|k}^{(j)}\right)$
\end{algorithmic}
\rule{\textwidth}{0.5pt}
\end{table}

\section{Pseudocode for GGIWTPHD filter pruning, absorption and capping}
\begin{table}[ht]
\caption{Pseudocode for GGIWTPHD filter pruning, absorption and capping}
\rule{\textwidth}{0.5pt}
\begin{algorithmic}[1] \label{GGIWTreduction}
    \STATE \textbf{input:} GGIWT components $\left\{w_{k|k}^{(j)}, \xi_{k|k}^{(j)}\right\}_{j=1}^{J_{k|k}}$, a pruning threshold $T$, an absorption threshold $U$ and a maximum number of allowed components $M$.
    \STATE \textbf{init:} Set $\ell \gets 0$ and $I \gets \left\{ i=1,...,J_{k|k} \big| w^{(i)}_{k|k} > T ~\land~ \frac{\alpha^{(i)}_{k|k}}{\beta^{(i)}_{k|k}} > 1 \right\}$
    \REPEAT 
        \STATE{$\ell \gets \ell + 1$}
        \STATE{$j \gets \underset{i\in I}{\arg\max} ~ w^{(i)}_{k|k}$}
        \STATE{$L \leftarrow\left\{i \in I \Big|\left(m_{k|k}^{(i)}-m_{k|k}^{(j)}\right)^{\mathsf{T}}\left(P_{k|k}^{(j)}\right)^{-1}\left(m_{k|k}^{(i)}-m_{k|k}^{(j)}\right) \leq U\right\}$}
        \STATE{$\tilde{w}_{k|k}^{(\ell)} \leftarrow \sum_{i \in L} w_{k|k}^{(i)}$}
        \STATE $\tilde{\xi}^{(\ell)}_{k|k} = \xi^{(j)}_{k|k}$
        \STATE{$I \gets I\setminus L$}
        
    \UNTIL{$I = \emptyset$}
    \STATE If $\ell > M$ then replace $\left\{\tilde{w}_{k|k}^{(j)}, \tilde{\alpha}_{k|k}^{(j)}, \tilde{\beta}_{k|k}^{(j)}, \tilde{m}_{k|k}^{(j)}, \tilde{P}_{k|k}^{(j)}, \tilde{\nu}_{k|k}^{(j)}, \tilde{V}_{k|k}^{(j)}\right\}_{j=1}^{\ell}$ by those of the $M$ components with largest weights.
    \STATE \textbf{output:} $\left\{\tilde{w}_{k|k}^{(j)}, \tilde{\xi}_{k|k}^{(j)}\right\}_{j=1}^{\ell},\tilde{\xi}_{k|k}^{(j)}=\left(\tilde{\alpha}_{k|k}^{(j)}, \tilde{\beta}_{k|k}^{(j)}, \tilde{m}_{k|k}^{(j)}, \tilde{P}_{k|k}^{(j)}, \tilde{\nu}_{k|k}^{(j)}, \tilde{V}_{k|k}^{(j)}\right)$
\end{algorithmic}
\rule{\textwidth}{0.5pt}
\end{table}
